# Supplementary material for: Augmented Reality and Robotics: A Survey and Taxonomy for AR-enhanced Human-Robot Interaction and Robotic Interfaces
Source: arXiv:2203.03254 source file (2022-03-07)
Supplement: Supplementary file 1 [file 14-appendix-figure.tex]

% \ryo{Based on Tian's Coding > \url{https://docs.google.com/spreadsheets/d/104RoRu7mBZz3y_K0yxHEfI-abIKfPbHHO-E9dRcQ-sk/edit?usp=sharing} }

% \newcolumntype{P}[1]{>{\centering\arraybackslash}p{#1}}

\begin{table*}[t]
\centering
\caption*{Appendix Table: Citation list for figures}
\label{tab:full-list}
\TableFontSize
\begin{tabular}{ \TableConfig }
\TableHeader \\
\hline
Section 3 - Approaches & & \\
\textcolor{color1}{
Augment Robots
}
& &
\\
\textcolor{color1}{
$\rightarrow$ On-Body (Head/Eye)
}
& 117 &
VRoom~\cite{jones2021belonging}
---
\cite{jones2021belonging, groechel2019using, walker2018communicating, mourtzis2017augmented, urbani2018exploring, maly2016augmented, rosen2020communicating, jones2020vroom, chen2021pinpointfly, kasahara2013extouch, young2007robot, liu2018interactive, young2006mixed}
\\
\textcolor{color1}{
$\rightarrow$ On-Body (Handheld)
}
& 0 &
Cartoon Face~\cite{young2007robot}
---
\cite{young2007robot, cao2019v, kasahara2013extouch, gradmann2018augmented, frank2017mobile}
\\
\textcolor{color1}{
$\rightarrow$ On-Environment
}
& 23 &
Shape-shifting Walls~\cite{takashima2016study}
---
\cite{takashima2016study, leithinger2013sublimate, lindlbauer2016combining, gronbaek2020kirigamitable, darbar2019dronesar, andersen2016projecting, roudaut2013morphees, follmer2013inform, xiao2013mirrorfugue, takashima2013transformtable, everitt2017polysurface}
\\
\textcolor{color1}{
$\rightarrow$ On-Robot
}
& 3 &
Furhat~\cite{al2012furhat}
---
\cite{al2012furhat, yamada2017isphere, tobita2011floating, suzuki2016gushed, kasetani2015projection, scheible2013displaydrone, villanueva2021robotar}
\\
\textcolor{color2}{
Augment Surroundings
}
& &
\\
\textcolor{color2}{
$\rightarrow$ On-Body (Head/Eye)
}
& 143 &
RoMA~\cite{peng2018roma}
---
\cite{peng2018roma, cao2019ghostar, arevalo2021assisting, walker2018communicating, luebbers2019augmented, rosen2020communicating, liu2018interactive, young2006mixed, hoang2021virtual, walker2019robot, quintero2018robot, bambusek2019combining, ostanin2018interactive, hedayati2018improving}
\\
\textcolor{color2}{
$\rightarrow$ On-Body (Handheld)
}
& 0 &
Mobile AR Interface~\cite{frank2017mobile}
---
\cite{frank2017mobile, zollmann2014flyar, stadler2016augmented, muhammad2019creating, hiraki2019navigatorch}
\\
\textcolor{color2}{
$\rightarrow$ On-Environment
}
& 52 &
PATI~\cite{gao2019pati}
---
\cite{gao2019pati, hashimoto2011touchme, kato2009multi, guo2009touch, wistort2011tofudraw, ishii2009designing, suzuki2019shapebots, robert2012blended, andersen2016projecting, kojima2006augmented, bambusek2019combining, piumatti2017spatial, hiraki2016phygital}
\\
\textcolor{color2}{
$\rightarrow$ On-Robot
}
& 20 &
Self-Actuated Projector~\cite{elsharkawy2021uwb}
---
\cite{elsharkawy2021uwb, lingamaneni2017dronecast, robert2010exploring, kasetani2015projection, huy2017see, morita2020extension, villanueva2021robotar, ochiai2011homunculus, watanabe2015communicating, costa2015augmented, scheible2013displaydrone, linder2010luminar}
\\
\\
\hdashline
Section 4 - Robots & & \\
\textcolor{color3}{
Form Factors
}
& &
\\
\textcolor{color3}{
$\rightarrow$ Robotic Arms
}
& 88 &
AR Control of Robotic Arm~\cite{chen2020combination}
---
\cite{chen2020combination, hoang2021virtual, andersen2016projecting, gao2019pati, frank2017mobile, peng2018roma, quintero2018robot, makhataeva2019safety, rosen2020communicating, liu2018interactive, arevalo2021assisting, ostanin2018interactive, bambusek2019combining, luebbers2019augmented, ostanin2020human, gradmann2018augmented, dinh2017augmented, qian2019augmented, maly2016augmented, fuste2020kinetic, cao2019ghostar, arevalo2020there, cha2018effects}
\\
\textcolor{color3}{
$\rightarrow$ Drones
}
& 20 &
DroneSAR~\cite{darbar2019dronesar}
---
\cite{darbar2019dronesar, walker2018communicating, lingamaneni2017dronecast, yamada2017isphere, walker2019robot, zollmann2014flyar, aleotti2017detection, chen2021pinpointfly, yuan2019human, hedayati2018improving, papachristos2016augmented, scheible2013displaydrone, cauchard2019drone, tobita2011floating, erat2018drone}
\\
\textcolor{color3}{
$\rightarrow$ Mobile Robots
}
& 98 &
Mobile Robot Path Planning~\cite{wu2020mixed}
---
\cite{wu2020mixed, costa2015augmented, elsharkawy2021uwb, stadler2016augmented, kojima2006augmented, wistort2011tofudraw, villanueva2021robotar, robert2010exploring, ishii2009designing, muhammad2019creating, ozgur2017cellulo, kasahara2013extouch, suzuki2016gushed, hashimoto2011touchme, guo2009touch, liu2011roboshop, kato2009multi, piumatti2017spatial, kasetani2015projection, cao2019v, hiraki2019navigatorch, jones2020vroom}
\\
\textcolor{color3}{
$\rightarrow$ Humanoid Robots
}
& 23 &
MR Interaction with Pepper~\cite{tran2021get}
---
\cite{tran2021get, al2012furhat, taher2015exploring, groechel2019using, rosen2020communicating, liu2018interactive, tran2020exploring, li2019augmented, arpaia2020robotic, howard2012using, cha2018effects}
\\
\textcolor{color3}{
$\rightarrow$ Vehicles
}
& 7 &
On-Vehicle Projector~\cite{ochiai2011homunculus}
---
\cite{ochiai2011homunculus, morita2020extension, watanabe2015communicating, korthauer2020watch, zolotas2018head, topliss2018establishing, nilwong2020outdoor, mercedes-f15, jaguar-rover}
\\
\textcolor{color3}{
$\rightarrow$ Actuated Objects
}
& 25 &
Actuated Pin Display~\cite{leithinger2011direct}
---
\cite{leithinger2011direct, lindlbauer2016combining, gronbaek2020kirigamitable, takashima2016study, leithinger2013sublimate, urbani2018exploring, follmer2013inform, leithinger2010relief, xiao2013mirrorfugue, xiao2016andantino, everitt2017polysurface, hardy2015shapeclip, everitt20193d}
\\
\textcolor{color3}{
$\rightarrow$ Combinations
}
& 0 &
Mobile Robotic Arm~\cite{de2019intuitive}
---
\cite{de2019intuitive, hashimoto2011touchme}
\todo{check more citations}

\\
\textcolor{color3}{
$\rightarrow$ Other Types
}
& 0 &
Augmented Laser Cutter~\cite{mueller2012interactive} 
---
\cite{mueller2012interactive, yamaoka2016mirageprinter, kapinus2019spatially, clemente2016humans, urbani2018exploring}
\todo{check more citations}
\\
\textcolor{color3}{
Relationship
}
& &
\\
\textcolor{color3}{
$\rightarrow$ 1 : 1
}
& 211 &
Common HRI~\cite{gradmann2018augmented} % AR Robot Operation with Tango
---
\cite{gradmann2018augmented, cardenas2021reducing, young2007robot, yuan2019human, chan2020augmented, walker2018communicating, evlampev2019obstacle, krupke2018comparison, zollmann2014flyar, leutert2013spatial, ni2017haptic, bambusek2019combining, reardon2018come, chen2021pinpointfly, lakshantha2014human, nawab2007joystick, frank2017mobile, quintero2018robot, kim2014task, arevalo2020there, pai2016virtual, diehl2020augmented, aschenbrenner2020mirrorlabs, leutert2012support}
\\
\textcolor{color3}{
$\rightarrow$ 1 : m
}
& 23 &
Swarm Robots~\cite{frank2017toward} % Toward Mobile MR with Multi-Robot Systems
---
\cite{frank2017toward, suzuki2019shapebots, hiraki2018phygital, le2016zooids, ozgur2017cellulo, kato2009multi, sugimoto2011robotable2, hiraki2019navigatorch, leitner2010physical, ghiringhelli2014interactive, guo2009touch, garcia2011educational}
\\
\textcolor{color3}{
$\rightarrow$ n : 1
}
& 18 &
Collaboration (Single Robot)~\cite{takashima2013transformtable} % TransformTable
---
\cite{takashima2013transformtable, pinciroli2018simulating, reina2015augmented, gronbaek2020kirigamitable, scheible2013displaydrone, nozaki2014flying, aschenbrenner2018comparing, magnenat2015enhancing, robert2012blended, elsharkawy2021uwb, park2018meet}
\\
\textcolor{color3}{
$\rightarrow$ n : m
}
& 8 &
Collaboration (Multiple Robots)~\cite{ozgur2017cellulo} % Cellulo
---
\cite{ozgur2017cellulo, takashima2016study, jost2018safe, kojima2006augmented, stein2019mixed, sugimoto2011mobile}
\\
\textcolor{color3}{
Scale
}
& &
\\
\textcolor{color3}{
$\rightarrow$ Handheld-scale
}
& 4 &
Handheld-scale~\cite{hiraki2015phygital} % Phigital Field
---
\cite{hiraki2015phygital, suzuki2019shapebots, lindlbauer2016combining, roudaut2013morphees, clemente2016humans, urbani2018exploring, ozgur2017cellulo}
\\
\textcolor{color3}{
$\rightarrow$ Tabletop-scale
}
& 44 &
Tabletop-scale~\cite{linder2010luminar} % LuminAR
---
\cite{linder2010luminar, pedersen2011tangible, guo2009touch, frank2016towards, lee2018physical, leithinger2011direct, follmer2013inform, jeong2018mechanism, leithinger2010relief, taher2015exploring, everitt2017polysurface, hardy2015shapeclip, aikawa2018comparison, al2012furhat, alrashidi2016pedagogical, carroll2013augmented, alrashidi2017evaluating, park2014qr, stadler2016augmented, calife2009robot, villanueva2021robotar, everitt20193d, kojima2006augmented, stein2019mixed, walker2019robot, fuste2020kinetic}
\\
\textcolor{color3}{
$\rightarrow$ Body-scale
}
& 166 &
Body-scale~\cite{materna2018interactive} % Interactive SAR in Collaborative Robot Programming
---
\cite{materna2018interactive, maly2016augmented, liu2018interactive, groechel2019using, peppoloni2015augmented, nishiwaki2008mixed, kobayashi2007overlay, taher2015exploring, williams2019mixed, ishii2009designing, lupetti2016designing, robert2010exploring, st2015robot, piumatti2017spatial, wistort2011tofudraw, prattico2019user, lamberti2019designing, lamberti2018robotquest, kasetani2015projection, arpaia2020robotic, park2019deep, rosen2020communicating, guhl2017concept}
\\
\textcolor{color3}{
$\rightarrow$ Building/City-scale
}
& 45 &
Building/City-scale~\cite{mercedes-f15}
---
\cite{mercedes-f15, yamada2017isphere, ochiai2011homunculus, jaguar-rover, watanabe2015communicating}
\\
\textcolor{color3}{
Proximity
}
& &
\\
\textcolor{color3}{
$\rightarrow$ Co-located
}
& 45 &
Co-located~\cite{de2019intuitive}
---
\cite{de2019intuitive, nowacka2013touchbugs, krzywinski2009robotable, xiao2013mirrorfugue, xiao2016andantino, robert2012blended, leithinger2011direct, pedersen2011tangible, gronbaek2020kirigamitable, takashima2013transformtable, ozgur2017cellulo, urbani2018exploring, everitt2017polysurface, hardy2015shapeclip, leithinger2013sublimate, aschenbrenner2018comparing, qian2020flexivision, christensen2017depth, sarai2017robot, matu2014stereoscopic, fong2019robot, luebbers2019augmented, ferraguti2020augmented, materna2018interactive}
\\
\textcolor{color3}{
$\rightarrow$ Co-located with Distance
}
& 175 &
Co-located with Distance~\cite{walker2019robot} % Robot Teleoperation with Virtual Surrogates
---
\cite{walker2019robot, darbar2019dronesar, hedayati2018improving, bambusek2019combining, de2019intuitive, gao2019pati, urbani2018exploring, luipers2021concept, gadre2019end, groechel2019using, nishiwaki2008mixed, gao2019fast, tran2021get, cousins2017development, dragone2007using, hiroi2010evaluation, shao2019development, estevez2015robot, young2007robot, hamilton2021s, dias2015augmented, ruiz2015immersive, qiu2020human, wu2018omnidirectional, williams2019mixed, wu2020mixed}
\\
\textcolor{color3}{
$\rightarrow$ Semi-Remote
}
& 14 &
Semi-Remote~\cite{erat2018drone} % Drone-Augmented Human Vision
---
\cite{erat2018drone, walker2018communicating, yuan2019human, chen2021pinpointfly, krzywinski2009robotable, huang2019flight, bentz2019unsupervised, aleotti2017detection, zollmann2014flyar, cauchard2019drone, chacko2020augmented, yamada2017isphere, scheible2013displaydrone, nozaki2014flying, tobita2011floating, guo2009touch}
\\
\textcolor{color3}{
$\rightarrow$ Remote
}
& 37 &
Remote~\cite{ruiz2015immersive} % Immersive displays for building spatial knowledge in multi-UAV operations
---
\cite{ruiz2015immersive, boeing-uav, hashimoto2011touchme, sugimoto2005time, tobita2011floating, gong2017real, peppoloni2015augmented, nuzzi2020hands, park2007teleoperation, dias2020deep, ni2017haptic, liu2011roboshop, kato2009multi}
\\
\\
\hdashline
Section 5 - Purposes & & \\
\textcolor{color4}{
Facilitate Programming
}
& 118 &
Collaborative Robot Programming~\cite{bambusek2019combining} % End-User Collaborative Robot Programming
---
\cite{bambusek2019combining, gao2019pati, liu2011roboshop, liu2018interactive, gradmann2018augmented, luebbers2019augmented, quintero2018robot, ostanin2018interactive, ostanin2020human, dinh2017augmented, cao2019v, fuste2020kinetic, cao2019ghostar, stadler2016augmented, guhl2017concept, gong2019projection, gadre2019end, frank2017mobile, frank2017toward, materna2018interactive, kapinus2020end, magnenat2015enhancing, sarai2017robot, ong2006methodologies, akan2011intuitive, araiza2019augmented, zou2018development, sugimoto2011robotable2, lambrecht2012spatial, ni2017haptic, chan2020towards, kain2017tablet, kapinus2019spatially, fang2009robot, lingamaneni2017dronecast}
\\
\textcolor{color4}{
Support Real-time Control
}
& 40 &
AR-supported Drone Navigation~\cite{zollmann2014flyar} % AR-supported Drone Navigation
---
\cite{zollmann2014flyar, ishii2009designing, frank2017mobile, cauchard2019drone, chen2021pinpointfly, aleotti2017detection, kasahara2013extouch, hiraki2019navigatorch, arevalo2020there, yuan2019human, guo2009touch, walker2019robot, hedayati2018improving, kato2009multi, hashimoto2011touchme, erat2018drone, cha2018effects, arevalo2021assisting, papachristos2016augmented, boeing-uav, clemente2016humans, wu2018omnidirectional, sosa2015imperfect, nawab2007joystick}
\\
\textcolor{color4}{
Improve Safety
}
& 21 &
Workspace Visualization~\cite{ostanin2020human} % Workspace Visualization
---
\cite{ostanin2020human, hoang2021virtual, makhataeva2019safety, chan2018virtual, chadalavada2020bi, jost2018safe, caruso2010robotic, boateng2021virtual}
\\
\textcolor{color4}{
Communicate Intent
}
& 66 &
Robot Arm Motion Intent~\cite{rosen2020communicating} % Robot Arm Motion Intent
---
\cite{rosen2020communicating, muhammad2019creating, huy2017see, ochiai2011homunculus, morita2020extension, watanabe2015communicating, andersen2016projecting, walker2018communicating, taher2015exploring, young2006mixed, villanueva2021robotar, chadalavada2020bi, williams2019mixed, tran2021get, reardon2019communicating, corotan2019indoor, yamaoka2016mirageprinter, korthauer2020watch, renner2018wysiwicd, arpaia2020robotic, gao2019fast, rozenberszki2021towards, lee2018augmented, reardon2018come}
\\
\textcolor{color4}{
Increase Expressiveness
}
& 97 &
AR Arms for Social Expression~\cite{groechel2019using} % MR Arms for Social Expression
---
\cite{groechel2019using, costa2015augmented, suzuki2016gushed, lindlbauer2016combining, piumatti2017spatial, kasetani2015projection, lee2018physical, takashima2016study, leithinger2013sublimate, pedersen2011tangible, al2012furhat, young2007robot, elsharkawy2021uwb, kojima2006augmented, robert2010exploring, robert2012blended, yamada2017isphere, gronbaek2020kirigamitable, darbar2019dronesar, jones2020vroom, tobita2011floating, wistort2011tofudraw, lingamaneni2017dronecast, scheible2013displaydrone, suzuki2019shapebots, ozgur2017cellulo, urbani2018exploring, hololens-robot, jones2021belonging, siu2018investigating, follmer2013inform, hiroi2010evaluation, hwang2008augmented, linder2010luminar}
\\
\\
\hdashline
Section 6 - Information & &
\\
\textcolor{color5}{
Internal Information
}
& 74 &
Internal Status~\cite{young2006mixed}, Robot's Capability~\cite{chakraborti2018projection}
% A Mixed Reality Approach to HumanRobot Interaction and Projection-Aware Task Planning
---
\cite{young2006mixed, chakraborti2018projection, groechel2019using, young2007robot, liu2018interactive, papachristos2016augmented, aleotti2017detection, makhataeva2019safety, mourtzis2017augmented, maly2016augmented, jia2020collision, clemente2016humans, xue2020enabling, de2019intuitive, ong2006methodologies, akinbiyi2006dynamic, alrashidi2016pedagogical, alrashidi2017evaluating, rozenberszki2021towards, dias2020deep, fang2009robot}
\\
\textcolor{color5}{
External Information
}
& 127 &
Object Status~\cite{andersen2016projecting}, Sensor/Camera Data~\cite{ruiz2015immersive}
---
\cite{andersen2016projecting, ruiz2015immersive, hedayati2018improving, boeing-uav, aleotti2017detection, liu2011roboshop, muhammad2019creating, papachristos2016augmented, erat2018drone, wu2020mixed, gradmann2018augmented, liu2020mobile, caiza2020augmented, huang2019flight, st2015robot, corotan2019indoor, materna2018interactive, livatino2010augmented, hiraki2016phygital, hoang2021virtual, chou2004augmented, livatino20113, dias2015augmented, bentz2019unsupervised, huang2020augmented, qiu2020human, zhang2020vision, mohareri2011autonomous, chen2020combination, gong2017real, williams2019mixed, gaschler2014intuitive, araiza2019augmented, kim2014task, nilwong2020outdoor, zou2018development, gong2019projection, hernandez2020increasing, luxenburger2019augmented, lamberti2019designing, lambrecht2012spatial, lee2018augmented, kain2017tablet}
\\
\textcolor{color5}{
Plan and Activity
}
& 111 &
Plan and Target~\cite{fuste2020kinetic}, Simulation~\cite{chen2021pinpointfly}
---
\cite{fuste2020kinetic, chen2021pinpointfly, walker2018communicating, huy2017see, ochiai2011homunculus, bambusek2019combining, yuan2019human, rosen2020communicating, magnenat2015enhancing, luebbers2019augmented, yamaoka2016mirageprinter, wistort2011tofudraw, guhl2017concept, frank2016towards, dinh2017augmented, muhammad2019creating, nuzzi2020hands, maly2016augmented, arpaia2020robotic, gao2019fast, malayjerdi2017mobile, chan2020augmented, evlampev2019obstacle, zollmann2014flyar, cao2018ani, arevalo2021assisting, xia2012augmented, ishii2009designing, reardon2019communicating, cao2019ghostar, kapinus2019spatially, kojima2006augmented}
\\
\textcolor{color5}{
Supplemental Content
}
& 94 &
Interactive Content~\cite{seifert2014hover}, Virtual Background~\cite{nintendo-mklive}
---
\cite{seifert2014hover, nintendo-mklive, jones2020vroom, siu2018investigating, piumatti2017spatial, robert2012blended, lindlbauer2016combining, leithinger2013sublimate, cauchard2019drone, arevalo2021assisting, suzuki2019shapebots, follmer2013inform, hartmann2020aar, garcia2011educational, sugimoto2005time, kapinus2020end, elsharkawy2021uwb, everitt20193d, shao2019development, costa2015augmented, cousins2017development, subin2017android, fong2019robot, calife2009robot, takashima2013transformtable, ro2019projection, everitt2017polysurface, chae2018pervasive, taher2015exploring, park2018meet, ruiz2015immersive, gronbaek2020kirigamitable, nozaki2014flying, suzuki2016gushed, yamada2017isphere, scheible2013displaydrone, park2019deep, tobita2011floating, takashima2016study, roudaut2013morphees, leithinger2011direct, leithinger2010relief}
\\
\\
\hdashline
Section 7 - Design & &
\\
\textcolor{color6}{
UIs and Widgets
}
& &
\\
\textcolor{color6}{
$\rightarrow$ Menus
}
& 0 &
Figure: \cite{cauchard2019drone, arevalo2021assisting}
---
\cite{cauchard2019drone, arevalo2021assisting, stadler2016augmented, dinh2017augmented, bambusek2019combining, gao2019pati, pedersen2011tangible, ostanin2020human, sugimoto2011robotable2, ostanin2018interactive, schmitt2021assisted}
\\
\textcolor{color6}{
$\rightarrow$ Information Panels
}
& 0 &
Figure: \cite{aleotti2017detection, ghiringhelli2014interactive}
---
\cite{aleotti2017detection, ghiringhelli2014interactive, urbani2018exploring, darbar2019dronesar, liu2018interactive, papachristos2016augmented, huang2020augmented}
\\
\textcolor{color6}{
$\rightarrow$ Labels and Annotations
}
& 0 &
Figure: \cite{darbar2019dronesar, zhu2016virtually}
---
\cite{darbar2019dronesar, zhu2016virtually, mourtzis2017augmented, urbani2018exploring, huy2017see}
\\
\textcolor{color6}{
$\rightarrow$ Controls and Handles
}
& 0 &
Figure: \cite{hashimoto2011touchme, pedersen2011tangible}
---
\cite{hashimoto2011touchme, pedersen2011tangible, sugimoto2011robotable2, wu2018omnidirectional, guo2009touch, frank2016towards, kapinus2019spatially}
\\
\textcolor{color6}{
$\rightarrow$ Monitors and Displays
}
& 0 &
Figure: \cite{hedayati2018improving, urbani2018exploring}
---
\cite{hedayati2018improving, urbani2018exploring, villanueva2021robotar, papachristos2016augmented, scheible2013displaydrone, nozaki2014flying, suzuki2016gushed, yamada2017isphere, qian2019augmented, darbar2019dronesar, cha2018effects}
\end{tabular}
\end{table*}

\begin{table*}[t]
\centering
\TableFontSize
\begin{tabular}{ \TableConfig }
\TableHeader \\
\hline
\\
\textcolor{color6}{
Spatial References and Visualizations
}
& &
\\
\textcolor{color6}{
$\rightarrow$ Points and Locations
}
& 0 &
Point References~\cite{quintero2018robot, tian2021adroid}, Landmarks~\cite{walker2019robot}, Control and Anchor Points~\cite{ostanin2018interactive}
---
\cite{quintero2018robot, tian2021adroid, walker2019robot, ostanin2018interactive, fuste2020kinetic, yuan2019human, el2021teaching, fung2011augmented, wu2020mixed, gaschler2014intuitive, alrashidi2016pedagogical, rotsidis2019improving, alrashidi2017evaluating}
\\
\textcolor{color6}{
$\rightarrow$ Paths and Trajectories
}
& 0 &
Simulated Trajectories~\cite{zollmann2014flyar, walker2018communicating, chen2021pinpointfly}, Connections and Relationships~\cite{kapinus2019spatially, fuste2020kinetic}
---
\cite{watanabe2015communicating, rosen2020communicating, gruenefeld2020mind, dinh2017augmented, zollmann2014flyar, walker2018communicating, chen2021pinpointfly, fuste2020kinetic, stadler2016augmented, chen2019pinpointfly, walker2019robot, lamberti2018robotquest, cha2018effects, dietrich2010visualization, kasahara2013extouch, luebbers2019augmented, park2021hands, diehl2020augmented, yamaoka2016mirageprinter, wistort2011tofudraw}
\\
\textcolor{color6}{
$\rightarrow$ Areas and Boundaries
}
& 0 &
Grouping~\cite{ghiringhelli2014interactive, ishii2009designing}, Bounding Box~\cite{hoang2021virtual}, Object Highlight~\cite{andersen2016projecting}
---
\cite{ghiringhelli2014interactive, ishii2009designing, hoang2021virtual, andersen2016projecting, chan2018virtual, dinh2017augmented, liu2011roboshop, estevez2015robot, gradmann2018augmented, ostanin2020human, frank2017mobile, mourtzis2017augmented, stadler2016augmented, bambusek2019combining}
\\
\textcolor{color6}{
$\rightarrow$ Other Visualizations
}
& 0 &
Force Map~\cite{kato2009multi, hiraki2019navigatorch}, Radar Map~\cite{omidshafiei2016measurable}, Color and Heat Map~\cite{makhataeva2019safety}
---
\cite{kato2009multi, hiraki2019navigatorch, omidshafiei2016measurable, makhataeva2019safety, hiraki2018phygital, arevalo2021assisting, papachristos2016augmented, muhammad2019creating, aleotti2017detection, cha2018effects, zollmann2014flyar, liu2018interactive, fuste2020kinetic}
\\
\textcolor{color6}{
Embedded Visual Effects
}
& &
\\
\textcolor{color6}{
$\rightarrow$ Anthropomorphic
}
& 0 &
Robot's Body~\cite{hololens-robot, groechel2019using}, Robot's Face~\cite{hiroi2010evaluation}, Human Body and Avatar~\cite{jones2020vroom, lee2018physical}, Character Animation~\cite{xiao2016andantino}
---
\cite{hololens-robot, groechel2019using, hiroi2010evaluation, jones2020vroom, lee2018physical, xiao2016andantino, walker2018communicating, al2012furhat, young2007robot, jones2021belonging, siu2018investigating, xiao2013mirrorfugue, aoki2005kobito, tobita2011floating}
\\
\textcolor{color6}{
$\rightarrow$ Virtual Replica
}
& 0 &
Robot's Virtual Replica~\cite{kasahara2013extouch, walker2019robot, guo2009touch}, Ghost Effects~\cite{rosen2020communicating}, Environment Replica~\cite{erat2018drone}, World in Miniature~\cite{boeing-uav}
---
\cite{kasahara2013extouch, walker2019robot, guo2009touch, rosen2020communicating, erat2018drone, boeing-uav, hashimoto2011touchme, chen2021pinpointfly, zollmann2014flyar, cao2019ghostar, bambusek2019combining, arevalo2020there, arevalo2021assisting, mourtzis2017augmented, qian2019augmented, maly2016augmented, stadler2016augmented, luebbers2019augmented, gradmann2018augmented, papachristos2016augmented, walker2018communicating, ostanin2020human, quintero2018robot, hoang2021virtual}
\\
\textcolor{color6}{
$\rightarrow$ Texture Mapping 
}
& 0 &
Texture Mapping based on Shapes\cite{nakagaki2016materiable, roudaut2013morphees, leithinger2011direct}, Supplemental Background Images~\cite{suzuki2019shapebots, ozgur2017cellulo, taher2015exploring}
---
\cite{nakagaki2016materiable, roudaut2013morphees, leithinger2011direct, suzuki2019shapebots, ozgur2017cellulo, taher2015exploring, follmer2013inform, hirai2018xslate, leithinger2010relief, everitt2017polysurface, lindlbauer2016combining, takashima2016study, leithinger2013sublimate, robert2012blended, robert2010exploring, pedersen2011tangible, jeong2018mechanism, gronbaek2020kirigamitable}
\\
\\
\hdashline
Section 8 - Interactions & &
\\
\textcolor{color7}{
Interactivity
}
& &
\\
\textcolor{color7}{
$\rightarrow$ Only Output
}
& 17 &
Programmed Visualization~\cite{walker2018communicating}
---
\cite{walker2018communicating, young2007robot, groechel2019using, suzuki2016gushed, tobita2011floating, scheible2013displaydrone, rosen2020communicating}
\\
\textcolor{color7}{
$\rightarrow$ Implicit
}
& 5 &
Proximity with Passerby~\cite{watanabe2015communicating}
---
\cite{watanabe2015communicating, subin2017android, qiu2020human, bentz2019unsupervised}
\\
\textcolor{color7}{
$\rightarrow$ Indirect
}
& 202 &
Body Gesture and Motion~\cite{piumatti2017spatial}
---
\cite{piumatti2017spatial, ostanin2018interactive, ishii2009designing, cao2019ghostar, walker2019robot, darbar2019dronesar, taher2015exploring, hedayati2018improving}
\\
\textcolor{color7}{
$\rightarrow$ Direct
}
& 43 &
Direct Physical Manipulation~\cite{nowacka2013touchbugs}
---
\cite{nowacka2013touchbugs, leithinger2013sublimate, guo2009touch, follmer2013inform, dietrich2010visualization, qian2019augmented, ozgur2017cellulo, lindlbauer2016combining}
\\
\textcolor{color7}{
Interaction Modalities
}
& &
\\
\textcolor{color7}{
$\rightarrow$ Tangible
}
& 58 &
Touch and Toy~\cite{guo2009touch}
---
\cite{guo2009touch, ozgur2017cellulo, lindlbauer2016combining, urbani2018exploring, robert2012blended, suzuki2019shapebots, leithinger2013sublimate, pedersen2011tangible, xiao2013mirrorfugue, xiao2016andantino, qian2019augmented, roudaut2013morphees}
\\
\textcolor{color7}{
$\rightarrow$ Touch
}
& 51 &
TouchMe~\cite{hashimoto2011touchme}
---
\cite{hashimoto2011touchme, kasahara2013extouch, gao2019pati, cao2019v, fuste2020kinetic, chen2021pinpointfly, gradmann2018augmented, stadler2016augmented, maly2016augmented, kato2009multi, gronbaek2020kirigamitable, guo2009touch, frank2017mobile, kain2017tablet}
\\
\textcolor{color7}{
$\rightarrow$ Controller
}
& 62 &
Laser-based Sketch~\cite{ishii2009designing} % Laser-based Sketch
---
\cite{ishii2009designing, hiraki2019navigatorch, wistort2011tofudraw, aleotti2017detection, robert2010exploring, hedayati2018improving, peng2018roma, walker2019robot, darbar2019dronesar, papachristos2016augmented}
\\
\textcolor{color7}{
$\rightarrow$ Gesture
}
& 79 &
Drone.io\cite{cauchard2019drone}
---
\cite{cauchard2019drone, quintero2018robot, erat2018drone, liu2018interactive, ostanin2018interactive, arevalo2021assisting, ostanin2020human, ochiai2011homunculus, luebbers2019augmented, bambusek2019combining, cha2018effects, dinh2017augmented, hololens-robot, siu2018investigating}
\\
\textcolor{color7}{
$\rightarrow$ Gaze
}
& 8 &
Gaze-driven Navigation~\cite{yuan2019human} % Gaze-driven Navigation
---
\cite{yuan2019human, morita2020extension, quintero2018robot, erat2018drone, taher2015exploring, ostanin2018interactive, liu2018interactive, arevalo2021assisting, argyle1976gaze, bambusek2019combining, chan2020augmented, park2021hands, ochiai2011homunculus, bentz2019unsupervised}
\\
\textcolor{color7}{
$\rightarrow$ Voice
}
& 11 &
Voice-based Control~\cite{huang2019flight}
---
\cite{huang2019flight, qian2019augmented, hoang2021virtual, jones2020vroom, tran2020exploring, arevalo2021assisting, dragone2007using, st2015robot, chan2020augmented, park2021hands, renner2018wysiwicd, al2012furhat, lee2011note, sosa2015imperfect, cardenas2021reducing}
\\
\textcolor{color7}{
$\rightarrow$ Proximity
}
& 14 &
Collision Avoidance~\cite{jost2018safe}
---
\cite{jost2018safe, wistort2011tofudraw, muhammad2019creating, watanabe2015communicating, takashima2016study, takashima2013transformtable, prattico2019user, lamberti2018robotquest}

\\
\textcolor{color8}{
Applications
}
& &
\\
\textcolor{color8}{
$\rightarrow$ Domestic and Everyday Use
}
&  &
{\it Household Task}
authoring home automation~\cite{el2021teaching, fung2011augmented, lakshantha2014human, seiger2017mixed, ishii2009designing, hiraki2019navigatorch, kato2009multi, cao2019v, liu2011roboshop, guo2009touch}, item movement and delivery~\cite{liu2020mobile, dragone2007using, kasahara2013extouch, chen2021pinpointfly}, multi-purpose table~\cite{takashima2013transformtable}
{\it  Photography}
drone photography~\cite{hedayati2018improving,erat2018drone}
{\it Advertisement}
mid-air advertisement~\cite{nozaki2014flying, scheible2013displaydrone, suzuki2016gushed, yamada2017isphere}
{\it Wearable Interactive Devices}
haptic interaction~\cite{urbani2018exploring}, fog screens~\cite{suzuki2016gushed}, head-worn projector for sharable AR scenes~\cite{hartmann2020aar}
{\it Assistance and companionship}
elder care~\cite{chae2018pervasive}, personal assistant~\cite{lee2011note, ro2019projection, renner2018wysiwicd}
{\it Tour and exhibition guide}
tour guide~\cite{mohareri2011autonomous}, museum exhibition guide~\cite{ro2019projection, hartmann2020aar}, guiding crowds~\cite{yamada2017isphere}, indoor building guide~\cite{corotan2019indoor}, museum interactive display~\cite{elsharkawy2021uwb}
\\
\\
\textcolor{color8}{
$\rightarrow$ Industry
}
&  &
{\it Manufacturing}
joint assembly and manufacturing~\cite{andersen2016projecting, boateng2021virtual, materna2018interactive, aschenbrenner2020mirrorlabs, ganesan2018better}, grasping and manipulation~\cite{chan2020augmented, huang2020augmented, gradmann2018augmented, chen2020combination, sarai2017robot}, tutorial and simulation~\cite{cao2018ani}, welding~\cite{ni2017haptic} 
{\it  Maintenance}
maintenance of robots~\cite{genccturk2019development, leutert2012support}, remote repair~\cite{calandra2021evaluating, aschenbrenner2018comparing}, performance monitoring~\cite{fong2019robot, filipenko2020virtual}, setup and calibration~\cite{nuzzi2020hands, puljiz2020hololens}, debugging~\cite{rotsidis2019improving}
{\it Safety and Inspection}
nuclear detection~\cite{aleotti2017detection}, drone monitoring~\cite{chen2021pinpointfly, erat2018drone, hedayati2018improving, yuan2019human}, safety feature~\cite{schmitt2021assisted, chakraborti2018projection, dietrich2010visualization, sarai2017robot, bolano2019transparent}, ground monitoring~\cite{kastner2019augmented, livatino2010augmented, young2006mixed}
{\it Automation and Teleoperation}
interactive programming interface~\cite{ong2006methodologies, frank2017toward, materna2017using, zou2018development, evlampev2019obstacle, fuste2020kinetic, hiraki2019navigatorch, luebbers2019augmented}
{\it Logistics}
package delivery~\cite{liu2020mobile}
{\it Aerospace}
surface exploration~\cite{cardenas2021reducing}, teleoperated manipulator~\cite{nawab2007joystick}, spacecraft maintenance~\cite{xia2012augmented}
\\
\\
\textcolor{color8}{
$\rightarrow$ Entertainment
}
&  &
{\it Games}
interactive treasure protection game~\cite{prattico2019user}, pong-like game~\cite{piumatti2017spatial, robert2010exploring}, labyrinth game~\cite{lindlbauer2016combining}, tangible game~\cite{hiraki2016phygital, lamberti2019designing, calife2009robot}, air hockey~\cite{walker2019robot, costa2015augmented}, tank battle~\cite{costa2015mixed, kojima2006augmented}, adventure game~\cite{carroll2013augmented}, role-play game~\cite{lamberti2018robotquest}, checker~\cite{lee2018physical}, domino~\cite{leitner2010physical}, ball target throwing game~\cite{park2019deep}, multiplayer game~\cite{estevez2015robot, sosa2015imperfect}, virtual playground~\cite{lupetti2016designing}
{\it  Storytelling}
immersive storytelling~\cite{shimizu2008mixed, robert2012blended, sugimoto2011mobile, wistort2011tofudraw, ozgur2017cellulo}
{\it Enhanced Display}
immersive gaming and digital media~\cite{takashima2016study}
{\it Music}
animated piano key press~\cite{xiao2016andantino, xiao2013mirrorfugue}, tangible tabletop music mixer~\cite{pedersen2011tangible}
{\it Festival}
festival greetings~\cite{scheible2013displaydrone}
{\it Aquarium}
robotic and virtual fish~\cite{lee2020realization}
\\
\\
\textcolor{color8}{
$\rightarrow$ Education and Training
}
&  &
{\it Remote Teaching}
remote live instruction~\cite{villanueva2021robotar}
{\it Training}
military training for working with robot teammates~\cite{jones2021ar}, piano instruction~\cite{xiao2016andantino, xiao2013mirrorfugue}, robotic environment setup~\cite{garcia2011educational}, robot assembly guide~\cite{alrashidi2016pedagogical}, driving review~\cite{aikawa2018comparison}, posture analysis and correction~\cite{tominaga2014around, howard2012using}
{\it Tangible Learning}
group activity~\cite{park2019deep, wistort2011tofudraw, magnenat2015enhancing, stein2019mixed, ozgur2017cellulo}, programming education~\cite{sugimoto2011robotable2}
\\
\\
\textcolor{color8}{
$\rightarrow$ Social Interaction
}
&  &
{\it Human-Robot Social Interaction}
reaction to human behaviors~\cite{cousins2017development, dragone2007using, subin2017android}, cartoon-art expression~\cite{young2007robot, ruiz2015immersive}, human-like robot head~\cite{al2012furhat}, co-eating~\cite{fujii2020development}, trust building~\cite{gao2019fast}, task assignment~\cite{tran2020exploring, tran2021get}
{\it Robot-Assisted Social Interaction}
projected text message conversations~\cite{scheible2013displaydrone}
{\it Inter-Robot Interaction}
human-like robot interaction~\cite{dragone2006mixing}
\\
\\
\textcolor{color8}{
$\rightarrow$ Design and Creativity Tasks
}
&  &
{\it Fabrication}
augmented 3D printer~\cite{yamaoka2016mirageprinter},interactive 3D modelling~\cite{peng2018roma}, augmented laser cutter~\cite{mueller2012interactive}, design simulation~\cite{cao2018ani}
{\it Design Tools}
circuit design guide~\cite{villanueva2021robotar}, robotic debugging interface~\cite{ghiringhelli2014interactive},  design and annotation tool~\cite{darbar2019dronesar}, augmenting physical 3D objects~\cite{kasetani2015projection}
{\it Theatre}
children’s play~\cite{ahn2013supporting}
\\
\\
\textcolor{color8}{
$\rightarrow$ Medical and Health
}
&  &
{\it Medical Assistance}
robotic-assisted surgery~\cite{wen2012robot, chou2004augmented, matu2014stereoscopic, qian2020flexivision, christensen2017depth, ferraguti2020augmented, akinbiyi2006dynamic, choi2013haptic, ho2020supervised, qian2019augmented}, doctors doing hospital rounds~\cite{lakshantha2014human}
{\it Accessibility}
robotic prostheses~\cite{clemente2016humans, fuste2020kinetic}
{\it Rehabilitation}
autism rehabilitation~\cite{arpaia2020robotic}, walking support~\cite{park2007teleoperation}
\\
\\
\textcolor{color8}{
$\rightarrow$ Remote Collaboration
}
&  &
{\it Remote Physical Synchronization}
physical manipulation by virtual avatar~\cite{lee2018physical}
{\it Avatar enhancement}
life-sized avatar~\cite{jones2020vroom}, floating avatar~\cite{tobita2011floating, yamada2017isphere}, life-sized avatar and surrounding objects~\cite{hwang2008augmented}
{\it Human-like embodiment}
traffic police~\cite{gong2017real}
\\
\\
\textcolor{color8}{
$\rightarrow$ Mobility and Transportation
}
&  &
{\it Human-vehicle interaction}
projected guidance~\cite{mercedes-f15, jaguar-rover}, interaction with pedestrians~\cite{chadalavada2020bi, ochiai2011homunculus}, display for passengers~\cite{korthauer2020watch}
{\it Augmented Wheelchair}
projecting intentions~\cite{watanabe2015communicating}, displaying virtual hands to convey intentions~\cite{morita2020extension}, self-navigating wheelchair~\cite{nilwong2020outdoor}, assistive features~\cite{zolotas2018head}
{\it Navigation}
tangible 3D map~\cite{lindlbauer2016combining}, automobile navigation~\cite{topliss2018establishing}
\\
\\
\textcolor{color8}{
$\rightarrow$ Search and Rescue
}
&  &
{\it Ground search}
collaborative ground search~\cite{reardon2019communicating}, target detection and notification~\cite{kastner2019augmented, wu2020mixed, livatino20113, muhammad2019creating, lee2018augmented, reardon2018come, livatino2010augmented, young2006mixed}, teleoperated ground search ~\cite{zhang2020vision, dias2015augmented, sugimoto2005time, wu2018omnidirectional, zalud2007augmented, livatino2021intuitive, cardenas2021reducing}
{\it Aerial search}
drone-assisted search and rescue~\cite{erat2018drone, papachristos2016augmented, yuan2019human}, target detection and highlight~\cite{williams2019mixed}
\\
\\
\textcolor{color8}{
$\rightarrow$ Workspace
}
&  &
{\it Adaptive Workspaces}
individual and collaborative workspace transformation~\cite{takashima2013transformtable, gronbaek2020kirigamitable, takashima2016study}
{\it Supporting Workers}
reducing workload for industrial robot programmers~\cite{stadler2016augmented}, mobile presentation~\cite{hartmann2020aar, park2018meet, linder2010luminar}, multitasking with reduced head turns~\cite{bentz2019unsupervised}, virtual object manipulation~\cite{qiu2020human}
\\
\\
\textcolor{color8}{
$\rightarrow$ Data Physicalization
}
&  &
{\it Physical Data Encoding}
physical bar charts~\cite{hardy2015shapeclip, taher2015exploring}, embedded physical 3D bar charts~\cite{suzuki2019shapebots}
{\it Scientific Physicalization}
mathematical visualization~\cite{follmer2013inform, leithinger2013sublimate}, terrain visualization~\cite{everitt20193d, everitt2017polysurface, leithinger2011direct, leithinger2013sublimate, nakagaki2016materiable}, medical data visualization~\cite{leithinger2013sublimate}
{\it , Physicalizing Digital Content}
handheld shape-changing display~\cite{lindlbauer2016combining, roudaut2013morphees}
\\

\end{tabular}
\end{table*}
